# Supplementary material for: SCOOP: Self-Supervised Correspondence and Optimization-Based Scene Flow
Source: arXiv:2211.14020 source file (2023-04-14)
Supplement: Supplementary file 1 [file failure.pdf]

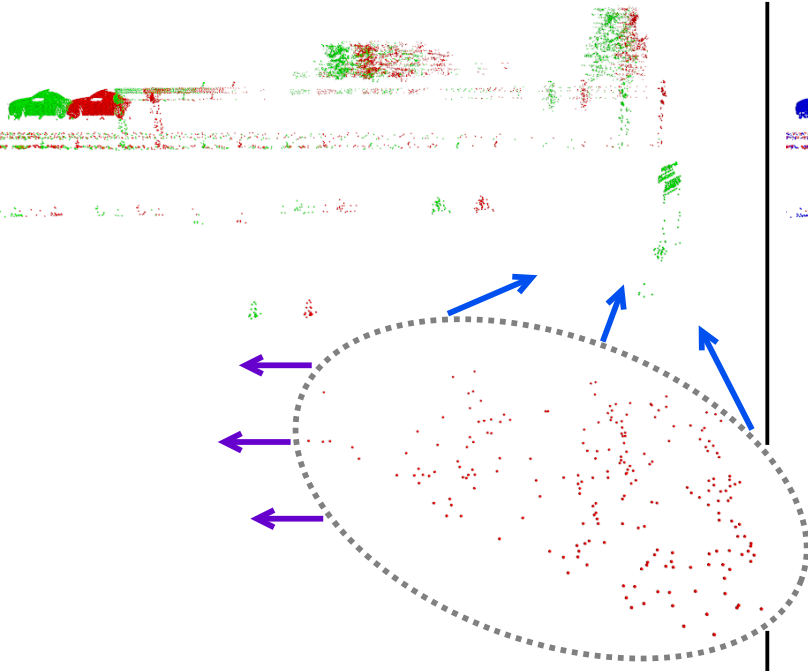

Input point clouds

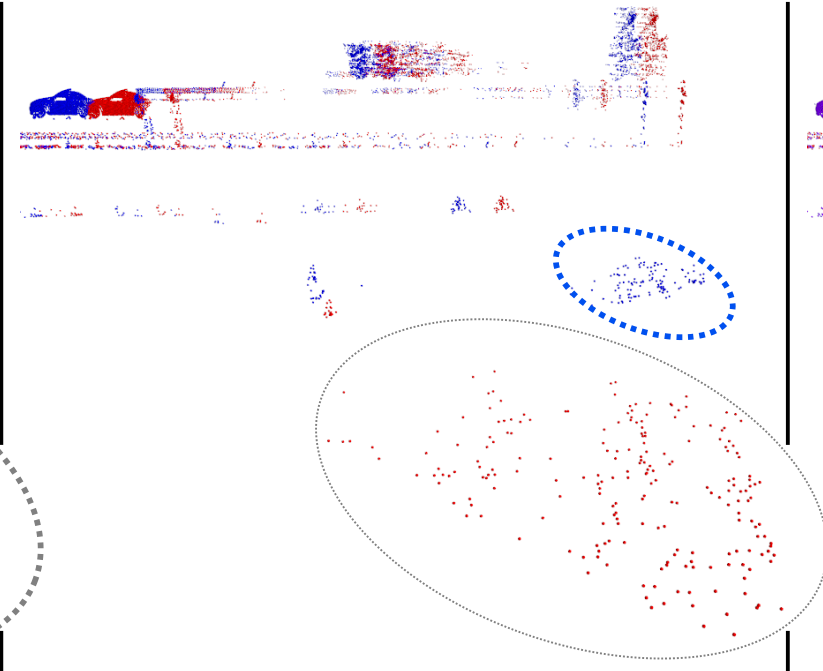

Warp by the estimated flow

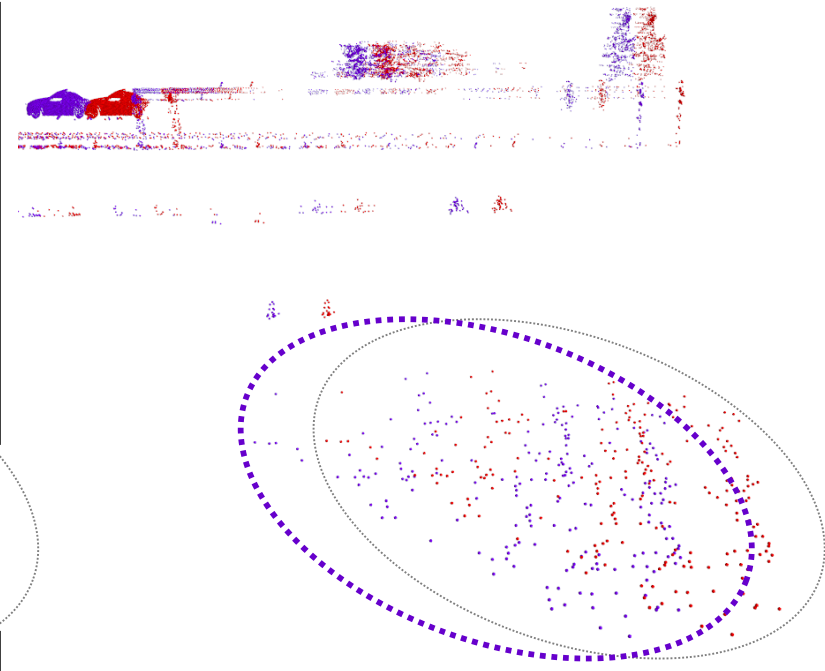

Warp by the ground-truth flow
